# Supplementary material for: Quantum and classical ripples in graphene
Source: arXiv:1712.08089 ancillary file (2018-04-10)
Supplement: Supplementary file 1 [file Supplemental-Material.pdf]

# Quantum and classical ripples in graphene
## *Supplemental Material*

Juraj Hašík,[1, 2, *] Erio Tosatti,[1, 3, 4] and Roman Martoňák[2]

[1] *International School for Advanced Studies (SISSA), Via Bonomea 265, I-34136 Trieste, Italy*
[2] *Department of Experimental Physics, Comenius University, Mlynská Dolina F2, 842 48 Bratislava, Slovakia*
[3] *CNR-IOM Democritos, Via Bonomea 265, I-34136 Trieste, Italy*
[4] *The Abdus Salam International Centre for Theoretical Physics (ICTP), Strada Costiera 11, I-34151 Trieste, Italy*

(Dated: April 10, 2018)

### COMPUTATIONAL METHODS

The membrane can be described by function $h(\vec{x})$ representing local height $h$ as function of internal 2D coordinates $\vec{x}$. We define the Fourier transform of the height as

$$h_{\vec{q}} = \frac{1}{N}\sum_j h_j \; e^{-i\vec{q}.\vec{x}_j} \tag{1}$$

where $\vec{x}_j$ refer to in-plane positions of atoms in the ideal graphene structure. The classical harmonic approximation then implies for small $q$ the relation $A\langle|h_q|^2\rangle = k_BT/\kappa q^4$, where $A$ is the area of the sample.

We model graphene by Tersoff's empirical potential[1], optimized for lattice dynamics and thermal transport[2]. Being much simpler than the reactive bond-order potential (Ref.[3]) but totally suitable for our defect-free studies, it provides a realistic harmonic description of all acoustic phonons of graphene, including the in-plane regular modes, the flexural branch with quadratic dispersion, and their interaction. By fitting the flexural phonon branch close to the $\Gamma$-point we obtain the value of bending rigidity $\kappa(T = 0K) = 1.82$ eV. The effective bending rigidity for finite $T$ can be extracted from the classical height-height correlation functions $\langle|h_q|^2\rangle$ and at low temperature $T = 0.6$ K we found $\kappa(T = 0.6K) = 1.83$ eV, in very good agreement with phonon calculation.

We implemented the constant pressure PIMC scheme along similar lines to those followed for 3D crystalline systems such as noble gas crystals of Ne and Ar[4] and polyethylene[5] (for review on PIMC see [6, 7]). The observables of the quantum system are obtained by sampling the corresponding classical system with effective Hamiltonian. We have used the primitive decomposition of the Hamiltonian, resulting in the effective Hamiltonian

$$H_M(\{\vec{r}_i^k\}) = \sum_{k=1}^{M}\sum_{i=1}^{N} \frac{m_i M}{2\hbar^2\beta^2}\left(\vec{r}_i^k - \vec{r}_i^{k-1}\right)^2 + \frac{1}{M}V(\{\vec{r}_i^k\})\ , \tag{2}$$

where $N$ is the number of particles in the quantum system, $m_i$ are their masses, $M$ is the Trotter number, $\beta = 1/k_BT$ is the inverse temperature and $V(\{\vec{r}_i\})$ is the potential energy of the system. Such an effective Hamiltonian represents a pseudo-classical system consisting of $M$ copies (Trotter slices) of the original system. The individual particles in neighboring Trotter slices are connected via harmonic "springs" with periodic boundary condition being applied along the Trotter direction, thus resembling a ring polymer. This pseudo-classical system has now $NM$ particles and can be simulated using the same constant pressure MC algorithm as in the classical case. The estimators for all configurational properties, diagonal in the coordinate representation, are straightforward analogues of their classical counterparts.

To sample the system, we have used four kinds of moves: chain moves, quantum moves, area moves and global wave moves. The chain move displaces uniformly all $M$ particles of a single ring polymer, which leaves the energy of the harmonic springs connecting them unchanged. This move samples the classical configurational phase space of the system. Quantum moves consisted of local translational moves of individual particles of the pseudo-classical system, which sample the quantum fluctuations around the classical paths. The in-plane area of the membrane is sampled by an isotropic scaling move, area move, which attempts to rescale the membrane in the $xy$-plane. Each area move consists of simultaneous rescaling of the simulation box and of $x$ and $y$ coordinates of all particles in all Trotter slices. Coordinates in the out-of-plane direction $z$ remain unchanged. The acceptance criterion for the move was based on the Boltzmann factor $s^{2NM}e^{-\beta E_M}$, where $E_M = H_M + pA_0s^2$, $p$ is the external tension, $A_0$ is the area of the reference

* jhasik@sissa.it

super-cell and $s$ is the scaling factor along the coordinate axes $x$ and $y$. In all simulations described in this paper, the external tension was set to zero. The last type of move, global wave move, is crucial to efficiently sample the long wavelength properties of the membrane [8]. In the single wave move $z$ coordinates of all particles of the pseudo-system are displaced according to a spatially periodic wave with given random wave vector $\vec{q}$ and amplitude $A$. Hence, for a given particle the attempted displacement is $\Delta z = A\cos(\vec{q}.\vec{r})$ for a cosine wave or $\Delta z = A\sin(\vec{q}.\vec{r})$ for a sine wave. One Monte Carlo step consisted of a random choice between performing the chain move for all ring polymers, the quantum move on each particle of the pseudo-classical system, the area move or the global wave move. The probabilities for selecting one of the aforementioned moves was chosen such that the ratio between frequency of these moves was 1 : 1 : 5 : 10. For all kinds of moves, their magnitudes were chosen to yield an acceptance ratio of 20 - 30 %. The graphene membrane is built up from $N_x \times N_y$ rectangular unit cells, each containing four carbons (two primitive cells). We have chosen $N_x$ and $N_y$ in order to have membranes of roughly square shape (Tab. I). For most of the simulations we performed $1.6 \times 10^6$ MC steps for equilibration and $8 \times 10^6$ MC steps for averaging. Observable quantities were sampled every 400 steps. Classical simulations were initialized from a flat membrane. The PIMC simulations were initialized from the final configurations of classical simulations, each Trotter slice being identical.

| N | $\mathbf{N_x \times N_y}$ | $\mathbf{L_x \times L_y}$ $[\AA \times \AA]$ |
|---|---|---|
| 4860 | 45 × 27 | 110.7 × 115.0 |
| 19440 | 90 × 54 | 221.4 × 230.0 |
| 108864 | 216 × 126 | 531.3 × 536.8 |

TABLE I: Dimensions of graphene membranes used in the simulations.

## FINITE SIZE EFFECTS AND TROTTER CONVERGENCE

In general, accessing lower temperatures by PIMC while preserving the accuracy requires increasing the number of Trotter slices and thus eventually makes this approach computationally prohibitive. However, as the Fig. 1 shows, even at temperature $T = 12.5$ K the height-height correlation functions of membranes of different size are practically identical. Therefore, to reach temperatures as low as $T = 0.6$ K we opt to simulate a smaller membrane with $N = 4860$ atoms which allowed us to increase the Trotter number up to $M = 432$. The total system size in this case was $4860 \times 432 \approx 2 \times 10^6$ atoms.

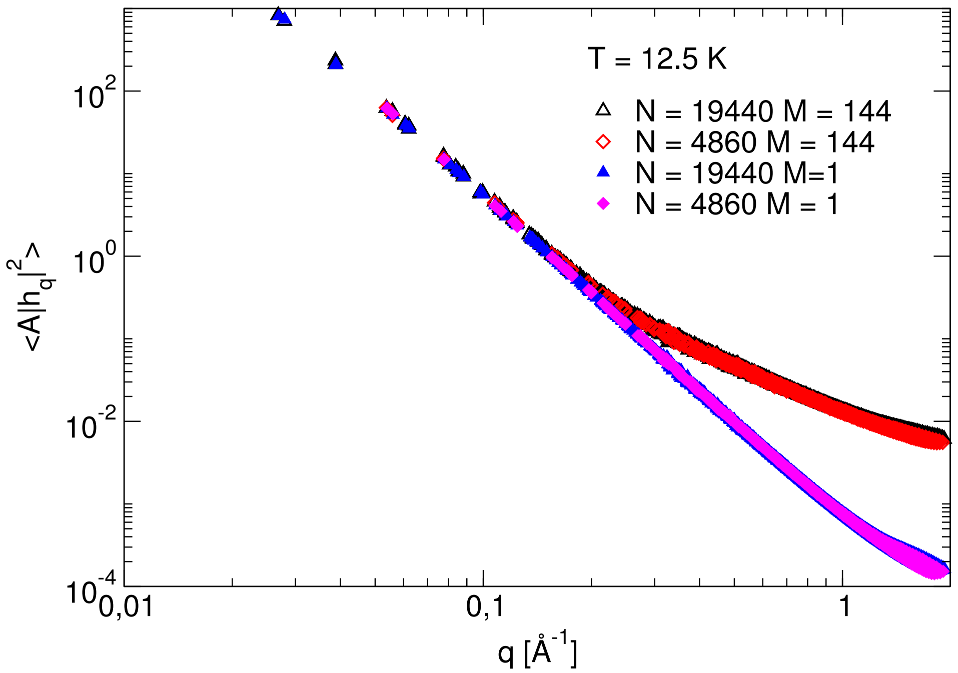


FIG. 1: Comparison of classical ($M = 1$) and quantum PIMC ($M = 144$) height-height correlation functions for two systems at temperature $T = 12.5$ K. The larger system has $N = 19440$ atoms and smaller one $N = 4860$ atoms.

For $N = 4860$ and $T = 5$ K the curves for different values of the Trotter number $M$ (Fig.2) show that already for relatively small $M$ the PIMC curves differ significantly from the classical curve for $q$-vectors larger than 0.1 Å$^{-1}$. Remarkably, convergence is fast for small and intermediate $q$ values while larger $M$ values are called for at larger $q$, see. e.g., the difference of $M$ =144 and 288. As also observed in Ref.[5] the soft degrees of freedom converge faster than the hard ones, that are intrinsically more quantum. Even though we could not keep the product $MT$ strictly constant down to the lowest temperature of $T = 0.6$ K, the convergence of the correlation function in the relevant region $q < 0.6$ Å$^{-1}$ is definitely sufficient as can be seen by comparing the curves for $M = 288$ and $M = 432$ (Fig.3).

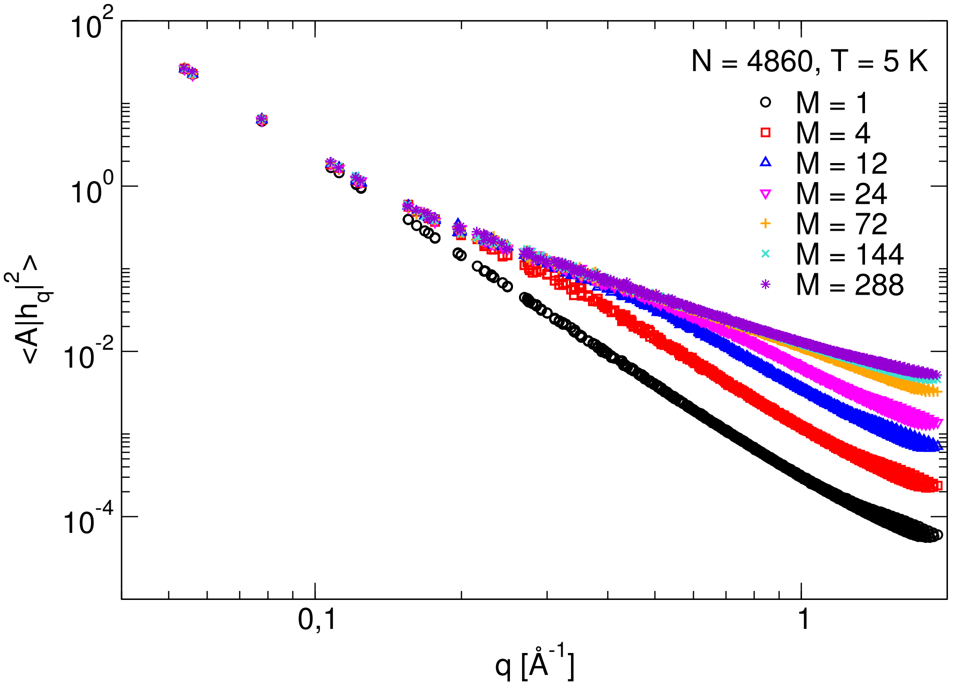


FIG. 2: Graphene PIMC height-height correlations for $N = 4860$ and $T = 5$ K for increasing values of the Trotter number $M$.

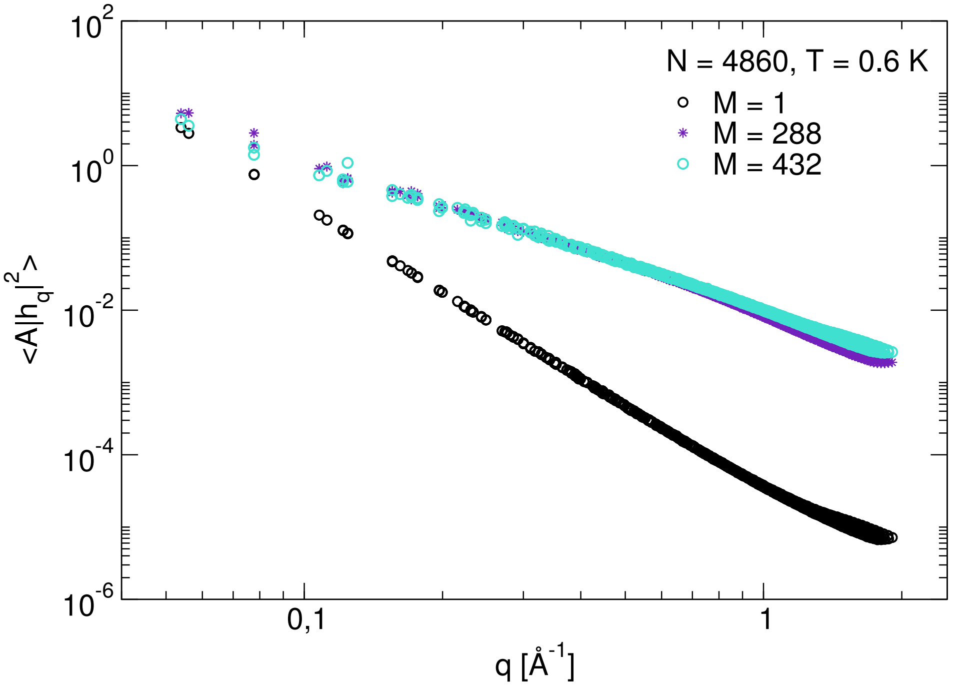


FIG. 3: Graphene PIMC height-height correlations for $N = 4860$ and $T = 0.6$ K for increasing values of the Trotter number $M$.

## CROSSOVER WAVELENGTH

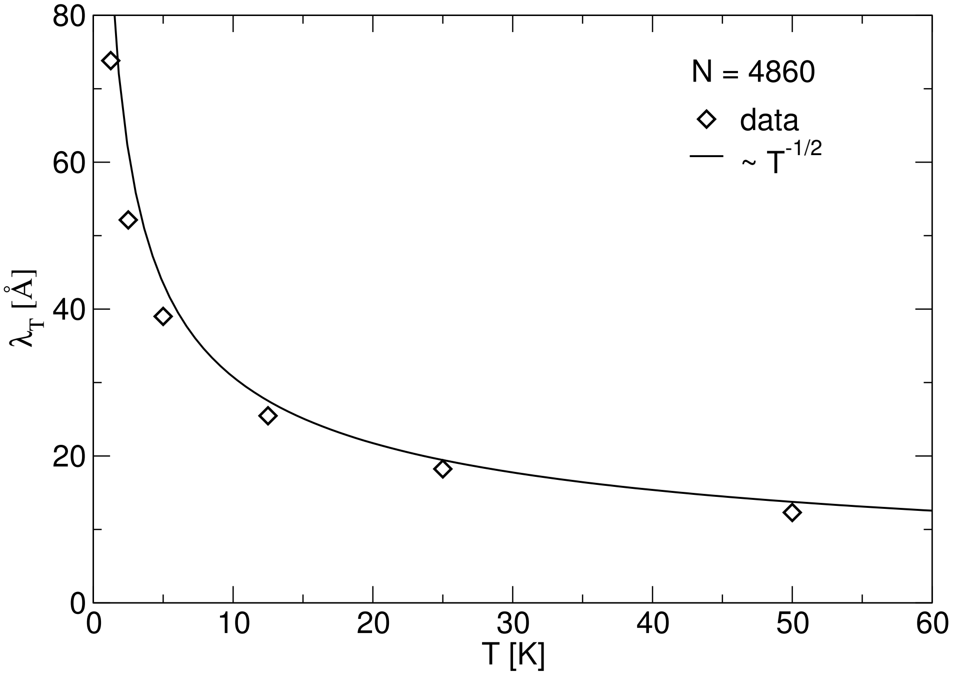


FIG. 4: Crossover wavelengths $\lambda_T = \frac{2\pi}{q_T}$ from PIMC simulations of graphene membrane with $N = 4860$ at low temperatures. Black solid line corresponds to the estimated $q_T$ for a membrane with bending rigidity $\kappa = 1.82$ eV.

## HISTOGRAM OF NORMAL ANGLES

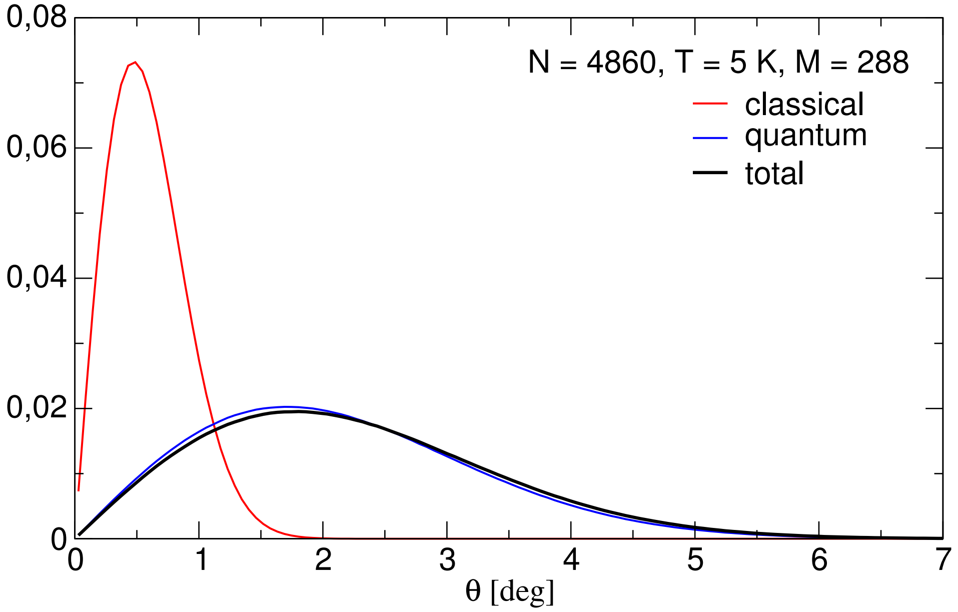


FIG. 5: Histogram of normal angles from PIMC simulation for $N = 4860$ at $T = 5$ K (including the $\sin\theta$ factor from the solid angle element).

[1] J. Tersoff, Phys. Rev. B **37**, 6991 (1988).
[2] L. Lindsay and D. A. Broido, Phys. Rev. B **81**, 205441 (2010).
[3] J. H. Los, L. M. Ghiringhelli, E. J. Meijer, and A. Fasolino, Phys. Rev. B **72**, 214102 (2005).
[4] M. H. Müser, P. Nielaba, and K. Binder, Phys. Rev. B **51**, 2723 (1995).
[5] R. Martoňák, W. Paul, and K. Binder, Phys. Rev. E **57**, 2425 (1998).
[6] D. M. Ceperley, Rev. Mod. Phys. **67**, 279 (1995).
[7] C. P. Herrero and R. Ramírez, J. Phys.: Condens. Matter **26**, 233201 (2014).
[8] J. H. Los, M. I. Katsnelson, O. V. Yazyev, K. V. Zakharchenko, and A. Fasolino, Phys. Rev. B **80**, 121405(R) (2009).
